# Supplementary material for: On Symmetry and the Reality of Holomorphic Hartree--Fock Wavefunctions
Source: arXiv:2012.12157 source file (2022-03-02)
Supplement: Supplementary file 3 [file oneelectronintegrals.tex]

\begin{tabular}{llll}
  \toprule
  Pathway & Constraining space & \multicolumn{2}{l}{One-electron integral coefficients}\\
  \midrule
  A
    & $\Psi\{\hat{s}_z, 0\}[\hat{i}]'$
    & $A_1^{-} = (x^2+1)\braket{1|\hat{h}|1} + 2x\braket{1|\hat{h}|3}$
    & $A_2^{-} = (x^2+1)\braket{1|\hat{h}|2} + 2x\braket{1|\hat{h}|4}$
  \\
   && $A_1^{+} = (y^2+1)\braket{1|\hat{h}|1} + 2y\braket{1|\hat{h}|3}$
    & $A_2^{+} = (y^2+1)\braket{1|\hat{h}|2} + 2y\braket{1|\hat{h}|4}$
  \\
  \addlinespace[6pt]
    & $\Psi\{\hat{s}_z, 0\}[\hat{\sigma}^{xz}]'$
    & $A_1^{-} = (x^2+1)\braket{1|\hat{h}|1} + 2x\braket{1|\hat{h}|4}$
    & $A_2^{-} = (x^2+1)\braket{1|\hat{h}|2} + 2x\braket{1|\hat{h}|3}$
  \\
   && $A_1^{+} = (y^2+1)\braket{1|\hat{h}|1} + 2y\braket{1|\hat{h}|4}$
    & $A_2^{+} = (y^2+1)\braket{1|\hat{h}|2} + 2y\braket{1|\hat{h}|3}$
  \\
  \addlinespace[12pt]
  B
    & $\Psi\{\hat{s}_z, 0\}[\hat{C}_2^{\clubsuit}]'$
    & $A_1^{-} = (x^2+1)\braket{1|\hat{h}|1} + 2x\braket{1|\hat{h}|3}$
    & $A_2^{-} = (x^2+1)\braket{1|\hat{h}|2} + 2x\braket{1|\hat{h}|4}$
  \\
   && $A_1^{+} = (y^2+1)\braket{1|\hat{h}|1} + 2y\braket{1|\hat{h}|3}$
    & $A_2^{+} = (y^2+1)\braket{1|\hat{h}|2} + 2y\braket{1|\hat{h}|4}$
  \\
  \bottomrule
\end{tabular}
