# Supplementary material for: On Symmetry and the Reality of Holomorphic Hartree--Fock Wavefunctions
Source: arXiv:2012.12157 source file (2022-03-02)
Supplement: Supplementary file 4 [file overlapintegrals.tex]

\begin{tabular}{llll}
  \toprule
  Pathway & Constraining space & \multicolumn{2}{l}{Overlap integral coefficients}\\
  \midrule
  A
    & $\Psi\{\hat{s}_z, 0\}[\hat{i}]'$
    & $S_1^{-} = \frac{1}{2}(x^2+1)\braket{1|1} + x\braket{1|3}$
    & $S_2^{-} = \frac{1}{2}(x^2+1)\braket{1|2} + x\braket{1|4}$
  \\
   && $S_1^{+} = \frac{1}{2}(y^2+1)\braket{1|1} + y\braket{1|3}$
    & $S_2^{+} = \frac{1}{2}(y^2+1)\braket{1|2} + y\braket{1|4}$
  \\
  \addlinespace[6pt]
    & $\Psi\{\hat{s}_z, 0\}[\hat{\sigma}^{xz}]'$
    & $S_1^{-} = \frac{1}{2}(x^2+1)\braket{1|1} + x\braket{1|4}$
    & $S_2^{-} = \frac{1}{2}(x^2+1)\braket{1|2} + x\braket{1|3}$
  \\
   && $S_1^{+} = \frac{1}{2}(y^2+1)\braket{1|1} + y\braket{1|4}$
    & $S_2^{+} = \frac{1}{2}(y^2+1)\braket{1|2} + y\braket{1|3}$
  \\
  \addlinespace[12pt]
  B
    & $\Psi\{\hat{s}_z, 0\}[\hat{C}_2^{\clubsuit}]'$
    & $S_1^{-} = \frac{1}{2}(x^2+1)\braket{1|1} + x\braket{1|3}$
    & $S_2^{-} = \frac{1}{2}(x^2+1)\braket{1|2} + x\braket{1|4}$
  \\
   && $S_1^{+} = \frac{1}{2}(y^2+1)\braket{1|1} + y\braket{1|3}$
    & $S_2^{+} = \frac{1}{2}(y^2+1)\braket{1|2} + y\braket{1|4}$
  \\
  \bottomrule
\end{tabular}
